# Supplementary material for: Argument Mining Driven Analysis of Peer-Reviews
Source: arXiv:2012.07743 source file (2020-12-10)
Supplement: Supplementary file 2 [file annotation_study_data_guideline.pdf]

# Annotation Guidelines<sup>1</sup>

## Definition

An argument is a reason given for supporting or attacking the acceptance of a review. It is either a direct support (or refutation) of the acceptance (direct argument) or a premise for another argument (indirect argument).

## Basic Criteria

We distinguish between two labels: **supporting acceptance (POS)** / **attacking acceptance (NEG)**. In this document, they are highlighted in green and red, separately.

A direct argument should satisfy the template 1 (T1):

The paper should be accepted/rejected, because (of) <argument >.

Example 1:

The paper should be accepted, because (of) <the platform was nicely designed and incorporated instant feedback and participator design elements> (graph20\_15\_1).

Example 2:

The paper should be rejected, because (of) <the research question is not clearly articulated> (graph20\_15\_1).

In the case of indirect arguments, it should satisfy the template 2 (T2):

<Another component> should be supported/attacked, because (of) <argument>.

Note that an indirect argument supporting a (direct) negative argument is negative as well.

Example 3

[Such an explanation (conjecture) is unconvincing]. [The study should have designed to gain more qualitative data to understand what factors affect their chat experience] (graph20\_17\_2).

Example 3 include two arguments. The former is a direct argument, which is supported by the latter.

---

<sup>1</sup> This document is based on Stab and Gurevych (2015) and Kluge.

The resulting sentence should be grammatically correct, whereas arguments may be non-clauses. To guarantee the correctness of grammar, we allow the substitution [you/the author]. In this context we see a suggestion as an argument, for instance:

Example 4:

The paper should be rejected, because <[the author] should explain or give intuition instead of simply referring to a different paper> (iclr19\_47\_1).

## Complementary Criteria

Generally, questions are non-argumentative since the answer is unknown. However, sometimes reviewers use rhetorical questions as argumentative device. These questions are not asked for the answer. On the contrary, the answer is clear according to the context. We annotate rhetorical questions as argument without using our templates<sup>2</sup>. Note that there's no clear boundary between question and rhetorical question. Our suggestion is that do not annotate a question if in doubt.

Example 5:

I am curious how the authors chose the 200ms timeout: [was there a pilot study run to determine how long the timeout should be]? [Did they record data during the studies which would allow them to empirically determine a superior timeout]? (graph20\_16\_3)

Example 6:

[It is also unclear how participatory design affected students learning experiences]. For example, [what were the practices and challenges that students had when playing the role of users of others designs]? [How had playing the role of users promoted or hindered learning]? (graph20\_15\_1)

The questions in Example 5 are non-argumentative since the answer from the author is expected. The two questions Example 6 attack the acceptance, since they are rhetorical indicating missing information in the experiment design.

## Tips

1. Indirect argument is always connected to the sentence directly before or after it.
2. Non-argumentative components are always explanations, which summarize the paper or describe the research background.

---

<sup>2</sup> We would not suggest ignoring questions generally, since rhetorical questions work as common argumentative device for scientific review. Reviewers used to use a chain of rhetorical questions as premises for a claim.

3. Make sure that the annotated components satisfy the grammatical correctness of templates.
4. If you split a sentence into two (or several) arguments, make sure that each argument guarantees the grammatical correctness of the templates.

Example 7:

Although [the platform was nicely designed and incorporated instant feedback and participator design elements] [...] (graph20\_15\_1).

Example 8:

Although [I am positive about the paper in general], [I do have the following concerns] (graph20\_4\_2).

Although Example 7 provides two reasons for accepting the paper, it should be annotated as whole, because the part after “and” cannot be filled in T1. On the other hand, Example 8 can be split into two arguments.

5. Generally, shell language, which guides the reader through the author’s argumentation structure should not be annotated. Typical shell expressions are: "As can be seen", "Another important reason is", “I agree/think/guess” etc. However, shell language should be included in the annotation if it contains a negation, e.g. "I disagree that".

## References

- Stab, Christian and Gurevych (2015): Guidelines for Annotating Argumentation Structures in Persuasive Essays. Version 1.2. [https://www.informatik.tu-darmstadt.de/ukp/research\\_6/data/argumentation\\_mining\\_1/argument\\_annotated\\_essays\\_version\\_2/index.en.jsp](https://www.informatik.tu-darmstadt.de/ukp/research_6/data/argumentation_mining_1/argument_annotated_essays_version_2/index.en.jsp). Accessed 29. Mai 2020.
- Kluge, Roland: Annotation Guidelines - Identifying Argumentation Structures in Controversial Educational Web Documents. [https://www.informatik.tu-darmstadt.de/media/ukp/data/fileupload\\_2/argument\\_annotated\\_news\\_articles/annotation\\_guidelinesArgMinNews.pdf](https://www.informatik.tu-darmstadt.de/media/ukp/data/fileupload_2/argument_annotated_news_articles/annotation_guidelinesArgMinNews.pdf). Accessed 29. Mai 2020.
